# Supplementary material for: Observational signatures of the dust size evolution in isolated galaxy simulations
Source: arXiv:2402.02659 source file (2024-07-25)
Supplement: Supplementary file 1 [file appendix.tex]

\section{Initial conditions of a NGC628-like galaxy}\label{Ap:morphological parameters of NGC628}
\section{Configuration dust mixes in \textsc{SKIRT}}
    dust opacity according to the dust grain size distributions of the gas particles. In SKIRT, we configure a plain power-law size distribution with an exponent of $4$ and adjust the opacity $\kappa_{c}$ by changing the weights $\omega_\mathrm{c}$ of each dust grain as follows
    \begin{eqnarray}
    \kappa_\mathrm{c} &=& \omega_\mathrm{c} * \kappa_\mathrm{c, \, 0}\\
    \omega_\mathrm{c} &=& \frac{d  \rho_d(a)}{d  a}N_\mathrm{c},
    \end{eqnarray}
    where  $\kappa_\mathrm{c, \, 0}$, $\frac{d  \rho_d(a)}{d  a}$, and $N_\mathrm{c}$ represent the opacity in the case of a power law size distribution with an exponent of $4$, the grain
    mass distribution of each gas particle, and the number of grain size bins ($N_\mathrm{c}=30$), respectively.
    The details is described in the tutorial of {\sc SKIRT}\footnote{\url{https://skirt.ugent.be/version9/_tutorial_custom_dust.html}}.
\section{Multi-bands images from edge-on view}
%\begin{figure*}
%        \includegraphics[width=1.0\textwidth]{Figure/MultiBandMapsEdgeOn.png}
%     \caption{fig: Multi-Band Maps Edge On}%
%     \label{fig: Multi-Band Maps Edge On}
%\end{figure*}
